# Supplementary material for: When to Stop Penalizing Actions? Martingale GRPO for VLA Reinforcement Learning
Source: arXiv:2610.32431 source file (2026-10-23)
Supplement: Supplementary file 1 [file contents.tex]

\makeatletter
\let\appendix@addcontentsline\addcontentsline
\renewcommand{\addcontentsline}[3]{%
  \appendix@addcontentsline{#1}{#2}{#3}%
  \def\appendix@stream{#1}%
  \def\appendix@toc{toc}%
  \ifx\appendix@stream\appendix@toc
    \addtocontents{atoc}{%
      \protect\contentsline{#2}{#3}{\thepage}{\@currentHref}%
      \protected@file@percent}%
  \fi
}

\pdfbookmark[0]{Appendix}{appendix.contents}
\begin{center}
  {\Large\bfseries Appendix\par}
\end{center}

\begingroup
  \definecolor{appendixcontentsblue}{RGB}{0,0,128}
  \hypersetup{linktoc=all}
  \let\ref\getrefnumber
  \setcounter{tocdepth}{2}
  \setlength{\parskip}{0pt}
  \renewcommand{\@dotsep}{2.5}
  \renewcommand*{\l@section}[2]{%
    \begingroup
      \renewcommand*{\numberline}[1]{%
        \hb@xt@\@tempdima{##1.\hfil}}%
      \@dottedtocline{1}{0em}{1.5em}%
        {\textcolor{appendixcontentsblue}{#1}}%
        {\textcolor{appendixcontentsblue}{#2}}%
    \endgroup
  }
  \renewcommand*{\l@subsection}[2]{%
    \@dottedtocline{2}{1.5em}{3em}%
      {\textcolor{appendixcontentsblue}{#1}}%
      {\textcolor{appendixcontentsblue}{#2}}%
  }
  \noindent{\large\bfseries Contents}\par\smallskip
  \@starttoc{atoc}
\endgroup
\bigskip
\makeatother
